# Supplementary material for: Structure, Thermodynamics, and Raman Spectroscopy of Rhenium-Doped Bulk MoS$_2$ from First Principles
Source: arXiv:2202.12889 ancillary file (2022-10-01)
Supplement: Supplementary file 1 [file SI.pdf]

# Supporting Information: Structure, Thermodynamics, and Raman Spectroscopy of Rhenium-Doped Bulk $MoS_2$ from First Principles

Enrique Guerrero* and David A. Strubbe*

*Department of Physics, University of California, Merced, Merced, CA 95343*

E-mail: eguerrero23@ucmerced.edu; dstrubbe@ucmerced.edu

**Table S1: Structural parameters**

| | Bond lengths (Å) | $a$, $b$, $c$ (Å) | $\alpha$, $\beta$, $\gamma$ (°) |
|---|---|---|---|
| $1 \times 1 \times 1$ | | | |
| Pristine | - | 3.191, 3.191, 12.415 | 90.0, 90.0, 120.0 |
| $2 \times 2 \times 1$ | | | |
| Mo-subst. | Re-S: 2.375×2, 2.414×2, 2.415×2 | 6.367, 6.382, 12.351 | 90.00, 90.00, 119.91 |
| t-intercal. | Re-S: 2.224, 2.226×2, 2.245 | 6.399, 6.399, 12.758 | 89.95, 90.05, 120.05 |
| S vacancy + intercal. | Re-S: 2.320×3 | 6.394, 6.394, 11.659 | 90.02, 89.99, 120.05 |
| o-intercal. | Re-S: 2.393×2, 2.395×4 | 6.372, 6.372, 12.671 | 90.04, 89.96, 120.08 |
| Mo-Re split interst. | Re-S: 2.222×3, Re-Mo: 2.249 | 6.541, 6.541, 12.466 | 90.00, 90.00, 120.00 |
| $2 \times 2 \times 2$ | | | |
| Mo-subst. | Re-S: 2.374×2, 2.415×2, 2.416×2 | 6.374, 6.382, 24.765 | 90.00, 90.00, 119.96 |
| t-intercal. | Re-S: 2.224, 2.226×2, 2.243 | 6.390, 6.390, 25.176 | 89.99, 90.01, 120.02 |
| S vacancy + intercal. | Re-S: 2.375, 2.405×2, 2.436×2 | 6.359, 6.359, 24.364 | 87.88, 92.12, 119.71 |
| o-intercal. | Re-S: 2.391×4, 2.400×2 | 6.378, 6.378, 25.079 | 90.07, 89.93, 120.02 |
| Mo-Re split interst. | Re-S: 2.211×3, Re-Mo: 2.252 | 6.462, 6.462, 24.903 | 90.00, 90.00, 119.99 |
| $3 \times 3 \times 1$ | | | |
| Mo-subst. | Re-S: 2.386×2, 2.394×4 | 9.584, 9.584, 12.367 | 90.00, 90.00, 120.04 |
| t-intercal.* | Re-S: 2.380×6 | 9.599, 9.598, 12.394 | 82.60, 97.40, 119.99 |
| S-subst. | Re-Mo: 2.706, 2.708×2 | 9.564, 9.564, 12.231 | 90.00, 90.01, 120.00 |
| o-intercal. | Re-S: 2.378, 2.379, 2.39×4 | 9.572, 9.580, 12.560 | 89.97, 89.82, 120.01 |
| Mo-Re split interst. | Re-S: 2.242, 2.246×2, Re-Mo: 2.261 | 9.656, 9.656, 12.471 | 90.00, 90.00, 119.91 |
| $4 \times 4 \times 1$ | | | |
| Mo-subst. | Re-S: 2.389×4, 2.392×2 | 12.775, 12.775, 12.385 | 90.00, 90.00, 119.94 |
| t-intercal. | Re-S: 2.217×3, 2.218 | 12.775, 12.775, 12.567 | 90.00, 90.00, 120.00 |
| S-subst. | Re-Mo: 2.701×3 | 12.756, 12.756, 12.313 | 90.00, 90.00, 120.00 |
| o-intercal. | Re-S: 2.383×4, 2.399×2 | 12.758, 12.758, 12.499 | 90.19, 89.81, 120.04 |
| Mo-Re split interst. | Re-S: 2.245×3, Re-Mo: 2.260 | 12.831, 12.830, 12.444 | 90.00, 90.00, 120.01 |

*The anomalous $3 \times 3 \times 1$ structure (Fig. S1) that was initialized as a t-intercalated structure relaxes to a 6-bond structure.

**Table S2: Formation energies (eV per $MoS_2$ unit)**

| | $2 \times 2 \times 1$ | $2 \times 2 \times 2$ | $3 \times 3 \times 1$ | $4 \times 4 \times 1$ |
|---|---|---|---|---|
| ($\mu_{\mathrm{Mo}} = \mu_{\mathrm{S}} = 0$) | | | | |
| Pristine | -2.616 | -2.616 | -2.616 | -2.616 |
| Mo-subst. | -2.273 | -2.444 | -2.461 | -2.529 |
| t-intercal. | -1.995 | -2.305 | -2.388 | -2.448 |
| S-subst. / S vacancy + intercal. | -1.792 | -2.218 | -2.250 | -2.408 |
| o-intercal. | -1.931 | -2.273 | -2.300 | -2.436 |
| Mo-Re split interst. | -1.911 | -2.249 | -2.318 | -2.447 |
| Mo-rich ($\mu_{\mathrm{Mo}} = -2.616$ eV, $\mu_{\mathrm{S}} = 0$) | | | | |
| Pristine | 0 | 0 | 0 | 0 |
| Mo-subst. | 0.015 | 0.008 | 0.009 | 0.005 |
| t-intercal. | 0.620 | 0.311 | 0.228 | 0.168 |
| S-subst. / S vacancy + intercal. | 0.823 | 0.398 | 0.370 | 0.208 |
| o-intercal. | 0.684 | 0.342 | 0.316 | 0.179 |
| Mo-Re split interst. | 0.705 | 0.367 | 0.297 | 0.168 |
| S-rich ($\mu_{\mathrm{Mo}} = 0, \mu_{\mathrm{S}} = -1.308$ eV) | | | | |
| Pristine | 0 | 0 | 0 | 0 |
| Mo-subst | 0.342 | 0.171 | 0.155 | 0.087 |
| t-intercal. | 0.620 | 0.311 | 0.228 | 0.168 |
| S-subst. / S vacancy + intercal. | 0.660 | 0.316 | 0.297 | 0.167 |
| o-intercal. | 0.684 | 0.342 | 0.316 | 0.179 |
| Mo-Re split interst. | 0.705 | 0.367 | 0.297 | 0.168 |

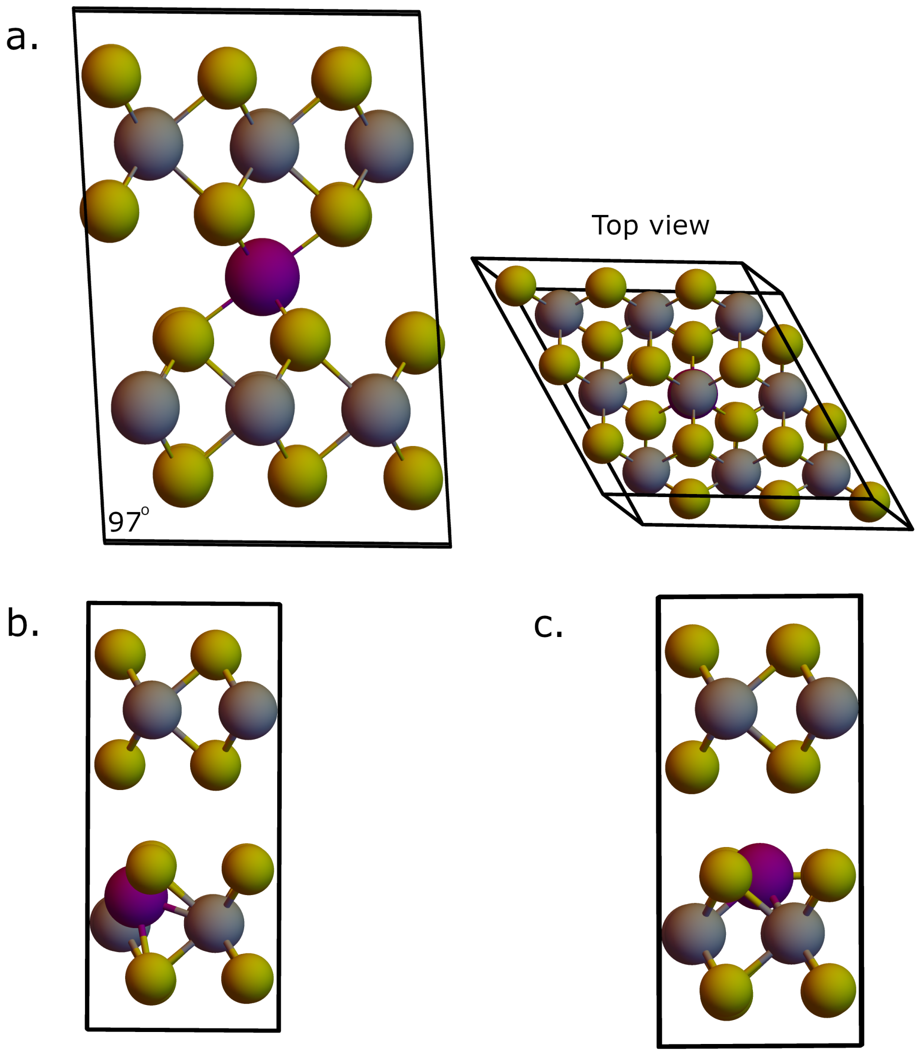


Figure S1: Further structures considered in this work. a) The anomalous $3 \times 3 \times 1$ supercell t-intercalated structure with non-standard stacking. The cell has angles of 82.60°, 97.40°, and 119.99° and a stacking pattern typically seen as a metastable stacking configuration of pristine $MoS_2$. b) The Mo-S bridge site where Re is initially placed between Mo and S; this structure relaxes to the Mo-Re split interstitial. c) The hollow-site structure where Re is placed in the center of three S atoms in a S-plane; this structure relaxes to o-intercalation.

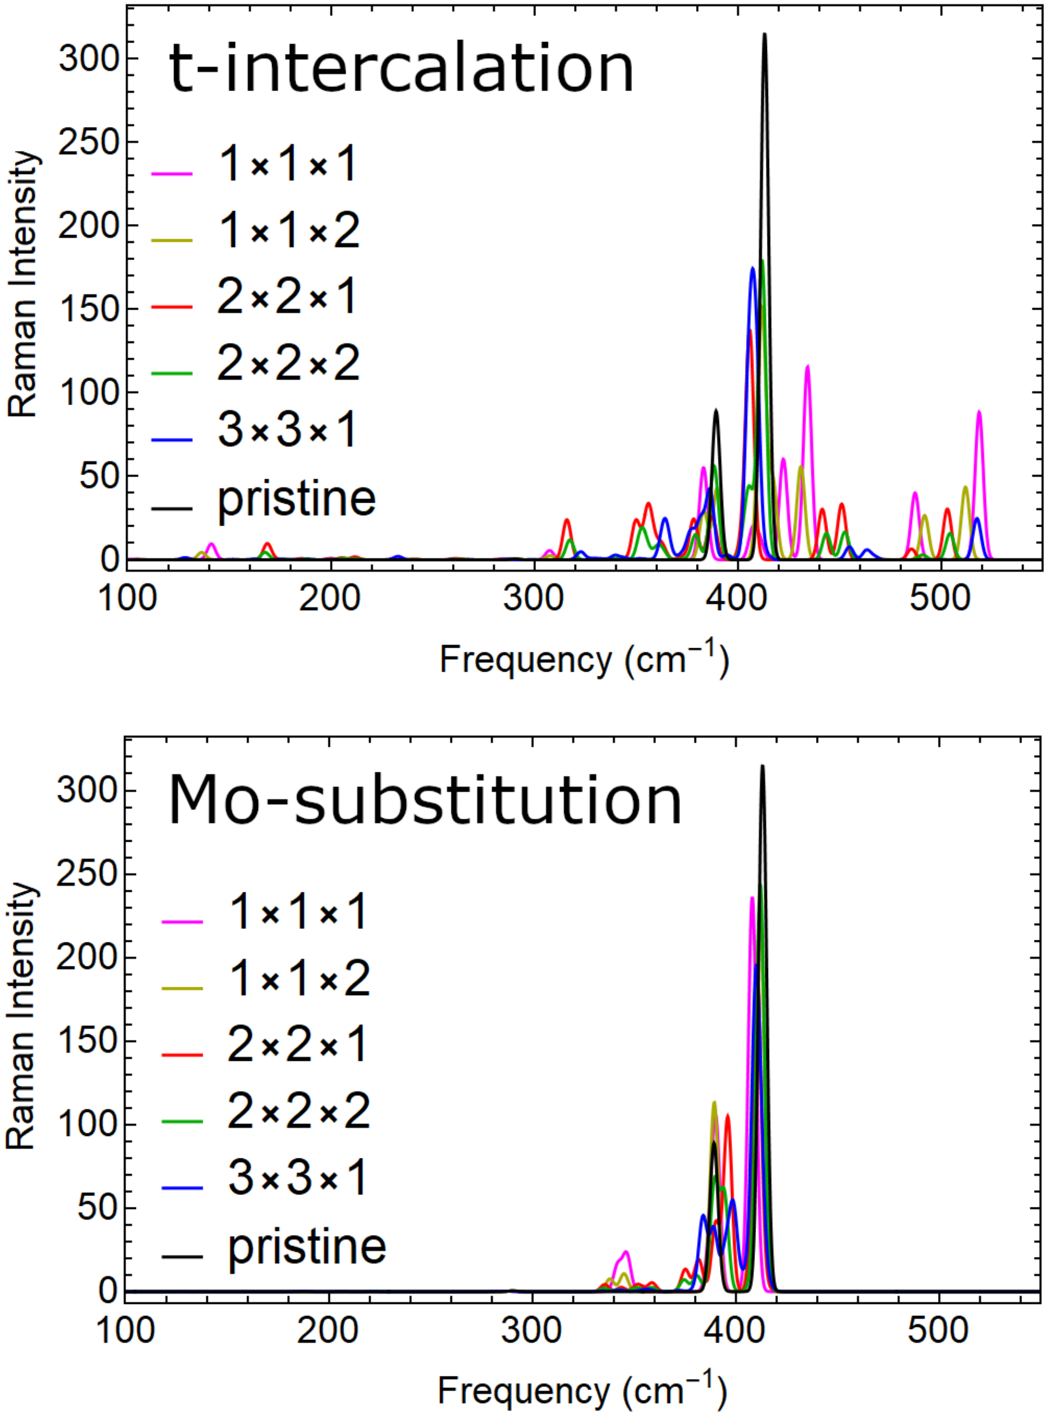


Figure S2: Full range of Raman spectra ($A^4$/amu per $MoS_2$ unit) of t-intercalated and Mo-substituted structures as computed by DFPT. We include $1 \times 1 \times 1$ and $1 \times 1 \times 2$ calculations (with $6 \times 6 \times 4$ and $6 \times 6 \times 2$ Monkhorst-Pack $k$-grids respectively).

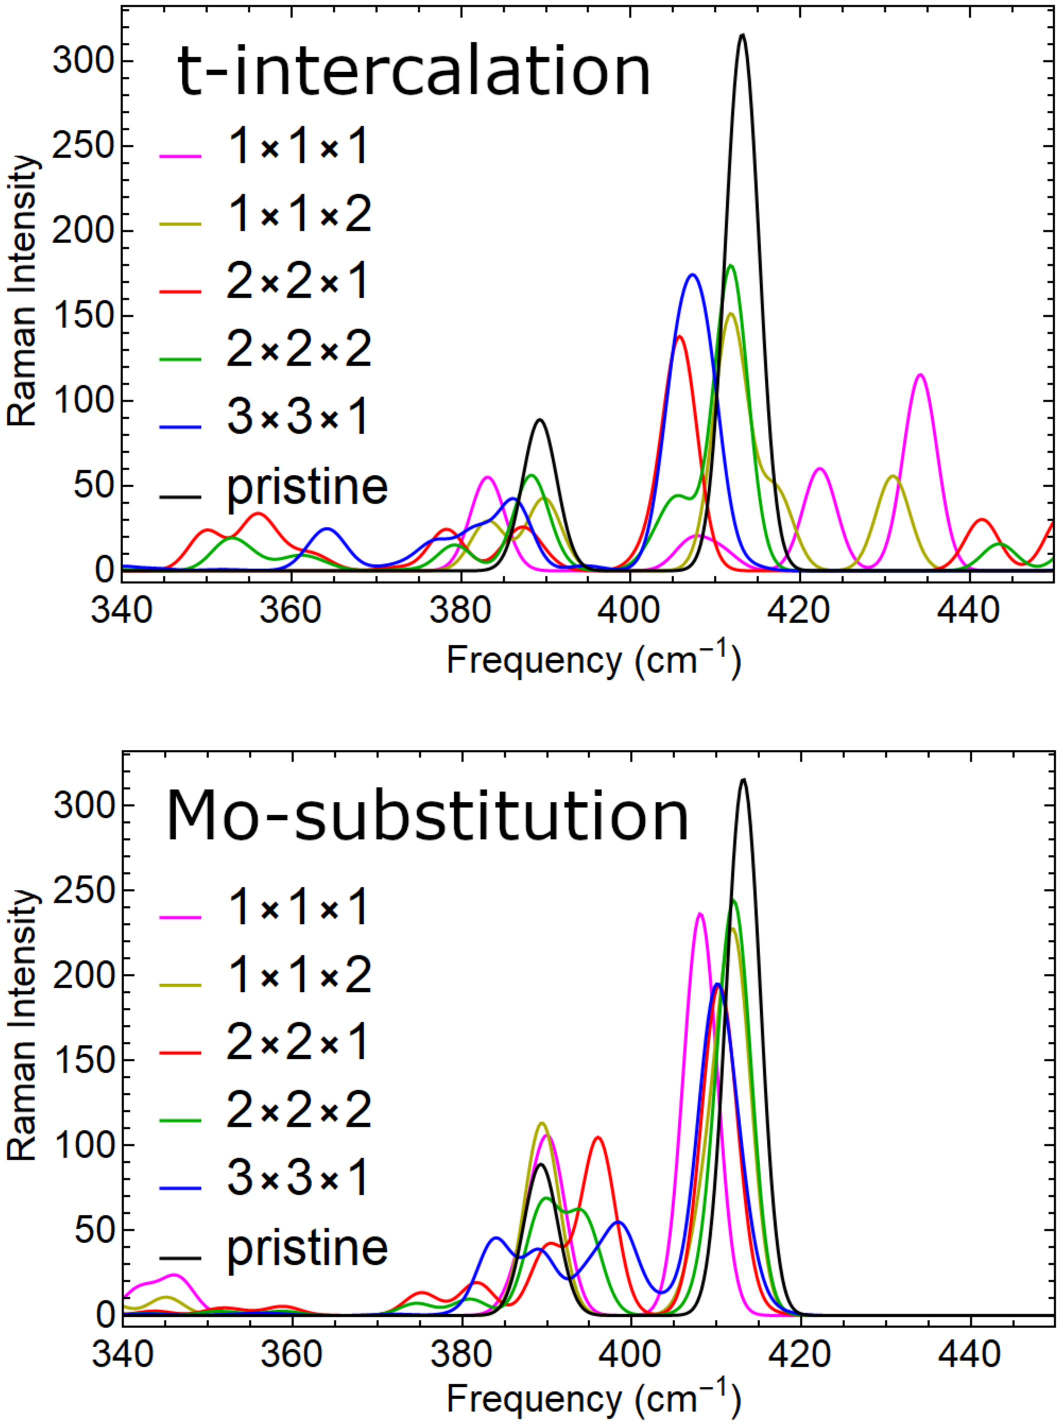


Figure S3: Detail of Fig. S2: Raman spectra (A$^4$/amu per $MoS_2$ unit) in the typically studied frequency range, of t-intercalated and Mo-substituted structures as computed by DFPT.

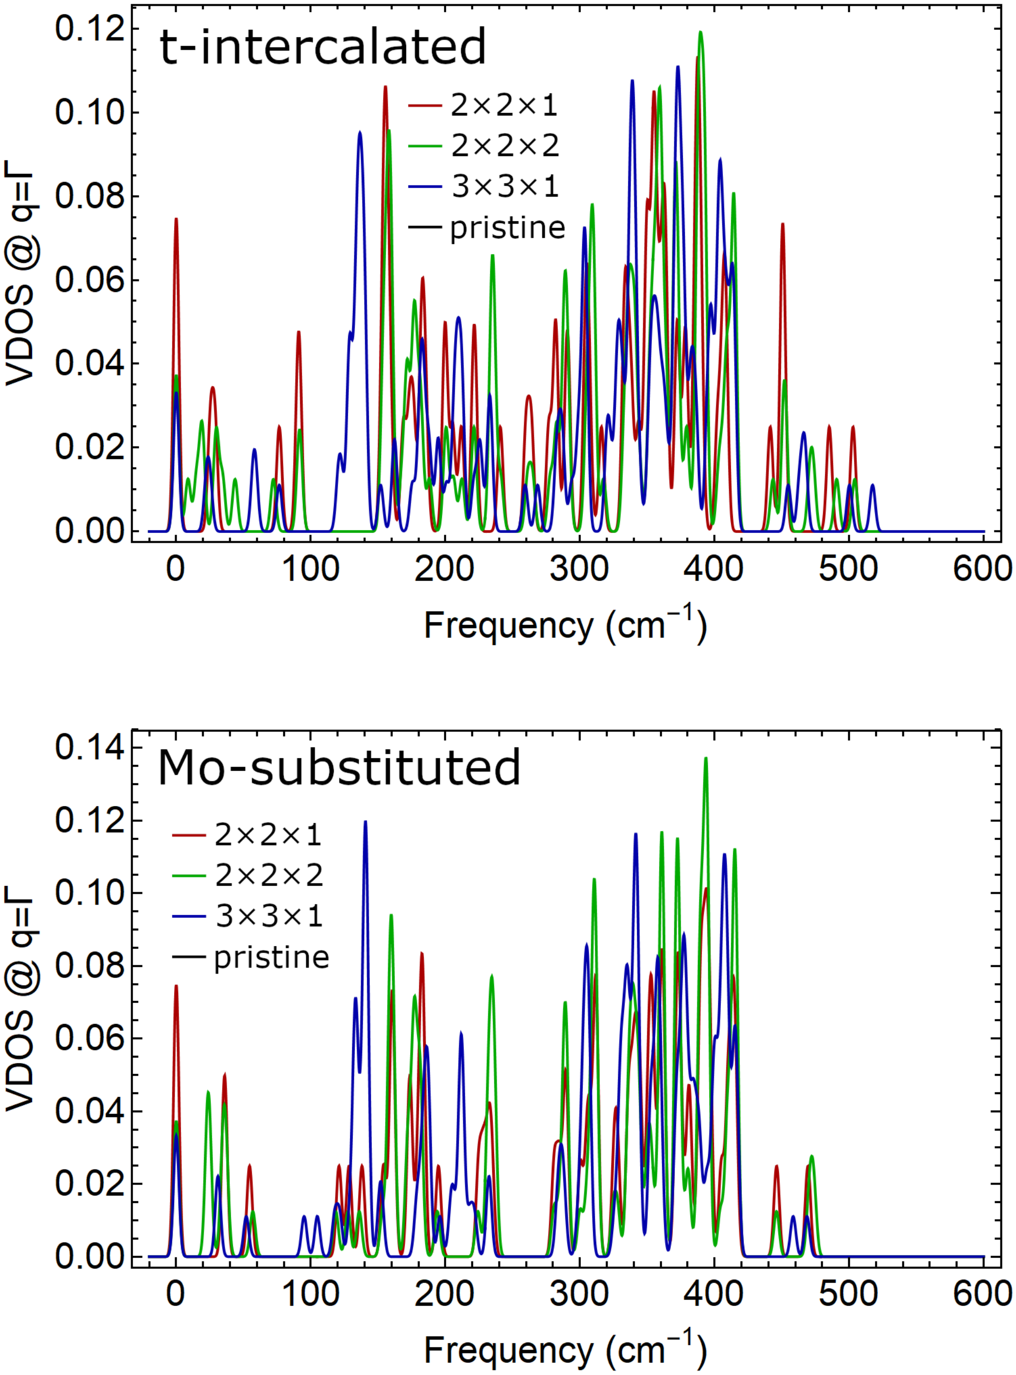


Figure S4: Vibrational density of states (VDOS) per $MoS_2$ unit at $q = \Gamma$ of t-intercalated and Mo-substituted structures as computed by DFPT.
